# Supplementary material for: No More Ambiguity in 360{\deg} Room Layout via Bi-Layout Estimation
Source: arXiv:2404.09993 source file (2024-04-15)
Supplement: Supplementary file 1 [file pretraining_supp.tex]

% Table generated by Excel2LaTeX from sheet 'Sheet1'
\begin{table*}
\centering
\vspace{4mm}
  \resizebox{0.8\linewidth}{!} % or it will overfull
  {
  \centering
    \begin{tabular}{lcccccc}
    \toprule
     & \multicolumn{2}{c}{Train From Scratch} & \multicolumn{2}{c}{ZInD-Simple Pretraining} & \multicolumn{2}{c}{ZInD-All Pretraining} \\
    \midrule
    Method & 2DIoU(\%) & 3DIoU(\%) & 2DIoU(\%) & 3DIoU(\%) & 2DIoU(\%) & 3DIoU(\%) \\
    \midrule
    LED${^2}$Net~\cite{wang2021led2} & 82.37 & 80.05 & 81.56 & 78.98 & 81.94 & 79.48 \\
    LGT-Net~\cite{jiang2022lgt} & 83.52 & 81.11 & 84.26 & 81.91 & 83.73 & 81.17 \\
    DOP-Net~\cite{shen2023dopnet} & 84.11 & 81.70  & 83.75 & 81.53 & 82.83 & 80.42 \\
    \midrule
    \rowcolor{ourcolor} 
    Ours (equivalent branch) & 84.56 & 82.05 & 84.17 & 82.01 & 84.49 & 82.24 \\
    % \midrule
    \rowcolor{ourcolor} 
    Ours (disambiguate) & \textbf{85.10} & \textbf{82.57} & \textbf{85.52} & \textbf{83.28} & \textbf{85.81} & \textbf{83.52} \\
    \bottomrule
    \end{tabular}%
  }
  \vspace{-2mm}
  \caption{\textbf{Pretraining Comparison.} For ZInD-Simple, we use their official checkpoints as pre-train models, then fine-tune and test on the MatterportLayout. For ZInD-All, }
  \vspace{-4mm}
  \label{tab:pretraining_supp}%
\end{table*}%
